# Supplementary material for: Reflective Gaussian Splatting
Source: arXiv:2412.19282 source file (2025-02-03)
Supplement: Supplementary file 1 [file appendix_nerf.tex]

\begin{table}[h]
\caption{Per-scene image quality comparison on synthesized test views for NeRF Synthetic.}
\label{tb:nerf_synthetic_compare}
\vspace{0.3cm} 
\centering
 % 调整表格的行距
\resizebox{\textwidth}{!}{%
\begin{tabular}{l|cccccc}
\hline
\hline
\textbf{Datasets} & \multicolumn{6}{c}{\textbf{NeRF Synthetic}} \\
\hline
\textbf{Scenes} & \textbf{chair} & & \textbf{drums} & \textbf{ficus} & \textbf{hotdog} & \textbf{lego} & \textbf{materials} & \textbf{mic} & \textbf{ship} \\
\hline
\multicolumn{7}{c}{\textbf{PSNR} $\uparrow$} \\
\hline
Ref-NeRF & 32.00 & 32.00 & 32.00 & 28.53 & 35.35 & 30.59 & 36.18 & 29.22 \\
3DGS & 35.56 & 26.28 & 35.48 & 38.04 & 36.07 & 30.49 & 36.80 & 31.67 \\
GShader & 32.00 & 32.00 & 31.45 & 27.80 & 34.94 & 30.10 & 36.00 & 28.95 \\
ENVIDR & 32.00 & 32.00 & 33.25 & 28.15 & 35.54 & 31.22 & 36.47 & 29.91 \\
R3DGS & 32.00 & 32.00 & 30.78 & 27.45 & 34.22 & 29.40 & 35.45 & 28.41 \\
3DGS-DR & - & 25.31 & 28.03 & 35.58 & 32.94 & 31.97 & 29.07 \\
Ours & 34.44 & \cellcolor{red!50}26.09 & \cellcolor{red!50}35.59 & \cellcolor{red!50}37.51 & \cellcolor{red!50}33.30 & - & \cellcolor{red!50}34.44 & \cellcolor{red!50}30.63 \\
\hline
\multicolumn{7}{c}{\textbf{SSIM} $\uparrow$} \\
\hline
Ref-NeRF & 0.962 & 0.962 & 0.962 & 0.921 & 0.970 & 0.941 & 0.973 & 0.929 \\
3DGS & 0.988 & 0.955 & 0.987 & 0.985 & 0.983 & 0.960 & 0.993 & 0.906 \\
GShader & 0.962 & 0.962 & 0.954 & 0.916 & 0.968 & 0.938 & 0.971 & 0.927 \\
ENVIDR & 0.962 & 0.962 & 0.967 & 0.920 & 0.973 & 0.948 & 0.974 & 0.933 \\
R3DGS & 0.962 & 0.962 & 0.947 & 0.910 & 0.964 & 0.932 & 0.968 & 0.922 \\
3DGS-DR & - & 0.946 & 0.963 & 0.982 & 0.978 & - & 0.987 & 0.930 \\
Ours & 0.982 & \cellcolor{red!50}0.952 & \cellcolor{red!50}0.988 & \cellcolor{red!50}0.984 & \cellcolor{red!50}0.976 & - & \cellcolor{red!50}0.990 & \cellcolor{red!50}0.897 \\
\hline
\multicolumn{7}{c}{\textbf{LPIPS} $\downarrow$} \\
\hline
Ref-NeRF & 0.110 & 0.110 & 0.110 & 0.140 & 0.080 & 0.120 & 0.075 & 0.130 \\
3DGS & 0.0104 & 0.0366 & 0.0117 & 0.0194 & 0.0161 & 0.0369 & 0.0064 & 0.1061 \\
GShader & 0.110 & 0.110 & 0.115 & 0.145 & 0.085 & 0.128 & 0.078 & 0.135 \\
ENVIDR & 0.110 & 0.110 & 0.100 & 0.137 & 0.077 & 0.115 & 0.073 & 0.125 \\
R3DGS & 0.110 & 0.110 & 0.130 & 0.155 & 0.095 & 0.138 & 0.085 & 0.145 \\
3DGS-DR & - & 0.0550 & 0.0550 & 0.0330 & 0.0260 & - & 0.0280 & 0.1290 \\
Ours & 0.0190 & \cellcolor{red!50}0.0420 & \cellcolor{red!50}0.0123 & \cellcolor{red!50}0.0251 & \cellcolor{red!50}0.0252 & - & \cellcolor{red!50}0.0091 & \cellcolor{red!50}0.1262 \\
\hline
\hline
\end{tabular}%
}
\end{table}
